# Supplementary material for: A Survey of Word Reordering in Statistical Machine Translation: Computational Models and Language Phenomena
Source: arXiv:1502.04938 source file (2016-03-14)
Supplement: Supplementary file 1 [file part-appendices.tex]

\appendixsection{Reordering constraints TODO}
\label{app:reoconstraints}

 \TOCHECK{TODO}

\noindent To avoid decoding dead-ends, the distortion limit has to be coupled with another constraint (gap constraint)
which ensures that the left-most uncovered input position~($\ell$) will still be reachable after translating the next source phrase.
Formally, to translate a new source interval $J_i$, the gap between $J_i$ and $\ell$ must not exceed the DL:
\begin{equation}\label{eq:gap-constraint}
 \left| \ell - \textrm{end}(J_{i}) -1 \right| \ \leq \textrm{DL}
\end{equation}

%%% 
\gap \TOCHECK{TODO}

\begin{itemize} \setlength{\itemsep}{.5mm}\setlength{\parskip}{.5mm} 
\item \textbf{MS (max skip)}: 
at each decoding step, translate one of the first \textit{k} uncovered source positions. In other terms, the translation of a limited number of words (at most \textit{k}) may be postponed indefinitely. 
\item \textbf{IS (inverted skip)}: at each decoding step, check how many source words after the first uncovered position \textit{j} have been translated. If they are less than $k{-}1$, translate any uncovered word, otherwise translate \textit{j}.
This means that the translation of at most $k{-}1$ source words can be anticipated at any point, while the rest of the sentence is covered monotonically.
\end{itemize}
The growth of the permutation search space for a sentence of 10 words, with respect to the threshold \textit{k} of the MS, IS and DL constraints is reported in Table \ref{tab:nb_perm}.%
\footnote{For a formal definition and complexity analysis of the DL and IBM constraints, we refer the reader to \namecite{Lopez:09}.} 
We notice that the space defined by DL is considerably smaller than the one defined by IBM constraints, as long as \textit{k} is small compared to the sentence length.
However, both types of constraint grow exponentially with \textit{k}.
The default configuration of the open-source PSMT toolkit Moses \cite{Koehn:07}
includes a DL of 6 words and this is widely accepted as a good baseline setting for many language pairs.

\begin{table}[t]
\setlength{\tabcolsep}{4pt}

\centering  \small
\begin{tabular}{l |r r r r r r r r r} 
\multicolumn{1}{c}{} & \multicolumn{9}{c}{Number of permutations (in thousands)}\\
\cline{1-10}
\ Threshold ($k$): 	& \multicolumn{1}{c}{2} & \multicolumn{1}{c}{3} & \multicolumn{1}{c}{4} & \multicolumn{1}{c}{5} & \multicolumn{1}{c}{6} & \multicolumn{1}{c}{7} & \multicolumn{1}{c}{8} & \multicolumn{1}{c}{9} &10$+$ \\
\hline
\ MS or IS	& 0.5 &	13   & 98 & 375   & 933 & 1729 & 2581 & 3266 & 3629 \\ 
\ DL 	& 0.2 & \ 3  & 24 & 128 & 476 & 1246 & 2333 & 3266 & 3629 \\ 
\hline
\end{tabular}
\caption{\label{tab:nb_perm} 
Number of permutations allowed for a 10-word sentence 
by the maximum skip (MS), inverted skip (IS) and distortion limit (DL) constraints,
while varying the respective thresholds ($k$). The total number of permutations is 10!=3,628,800.}
\end{table}

An enhancement to the IBM constraints was proposed by \namecite{Tillmann:03} 
to specifically address the reordering of verbs between German and English, in a word-based SMT system.
This paradigm allows to set different thresholds for the anticipation and for the postponement of some input words.
A reordering state is added to the decoder to ensure that any reordering pattern (either \textit{skip} or \textit{move}) is completed before initiating a new one. Both reordering patterns are strictly defined and, aside from them, decoding proceeds monotonically.
For the German-English translation direction, 
\namecite{Tillmann:03} manually set their thresholds so that one word may be skipped for at most 4 positions, and up to 2 words may be moved left by at most 10 positions. In this way, a non-contiguous verb chunk in German may be correctly reordered into a contiguous verb chunk in English.
Note, however, that these constraints do not take into account the actual position of the verbs in the input sentence.

%%% 

\COMMENT{
%We have already presented in equation~\eqref{eq:phr-disto} the \textbf{distortion cost} function, which is commonly employed as a basic reordering model by modern PSMT systems, such as Moses.
%
A weakness of this function is that it penalizes long jumps only when they are performed,
rather than accumulating their cost gradually.
As a result, hypotheses with gaps (\ie uncovered input positions) can proliferate and cause the pruning of more monotonic hypotheses that could lead to  overall better translations.%
To solve this problem, \namecite{Moore:07} proposed an improved version of the distortion cost function
which consists in ``incorporating an estimate of the distortion penalty yet to be incurred into the estimated score for the
portion of the source sentence remaining to be translated'' (\textbf{early distortion cost}).%
\footnote{A similar idea had been proposed by \namecite{Och:04} for the alignment template SMT approach, under the name of min-jumps.}
This function has the same value as the standard one over a complete translation hypothesis, 
provided that the jump from the last translated word to the end of the sentence is taken into account.
As a difference, though, it anticipates the gradual accumulation of the total distortion cost,
making hypotheses with the same number of covered words more comparable with one another.
For instance, in Figure~\ref{fig:running-example-phr},
standard distortion becomes 1 when we skip the first source phrase $J_3$ 
but does not increase while we cover $J_1$ and $J_2$.
Only when we jump back and forth to cover $J_3$ and 
continue, the cost finally increases by +6 and +5 leading to a total of 12.
%
%On the contrary, early distortion cost always includes the minimal cost that will be incurred to cover all current gaps and return to the right-most covered position. 
On the contrary, early distortion is already 6 after the first step: that is, 1 for skipping $J_3$ plus 5 for the minimal future cost.
The second step is monotonic, but the minimal future cost is incremented by 6. 
When we finally jump back and forth to translate $J_3$ and continue, no additional cost is paid, leading to the same total of 12.
%Early distortion cost is computed by an algorithm that keeps track of the uncovered input positions and is available in Moses as a decoding option.
}

%%%%%%%%%%%%%%%%%%%%%%%%%
\appendixsection{Example of KRS computation}
\label{app:krs}

 \TOCHECK{TODO}

%%% EXAMPLE

\begin{figure}[h]
\centering
\includegraphics[width=.7\textwidth]{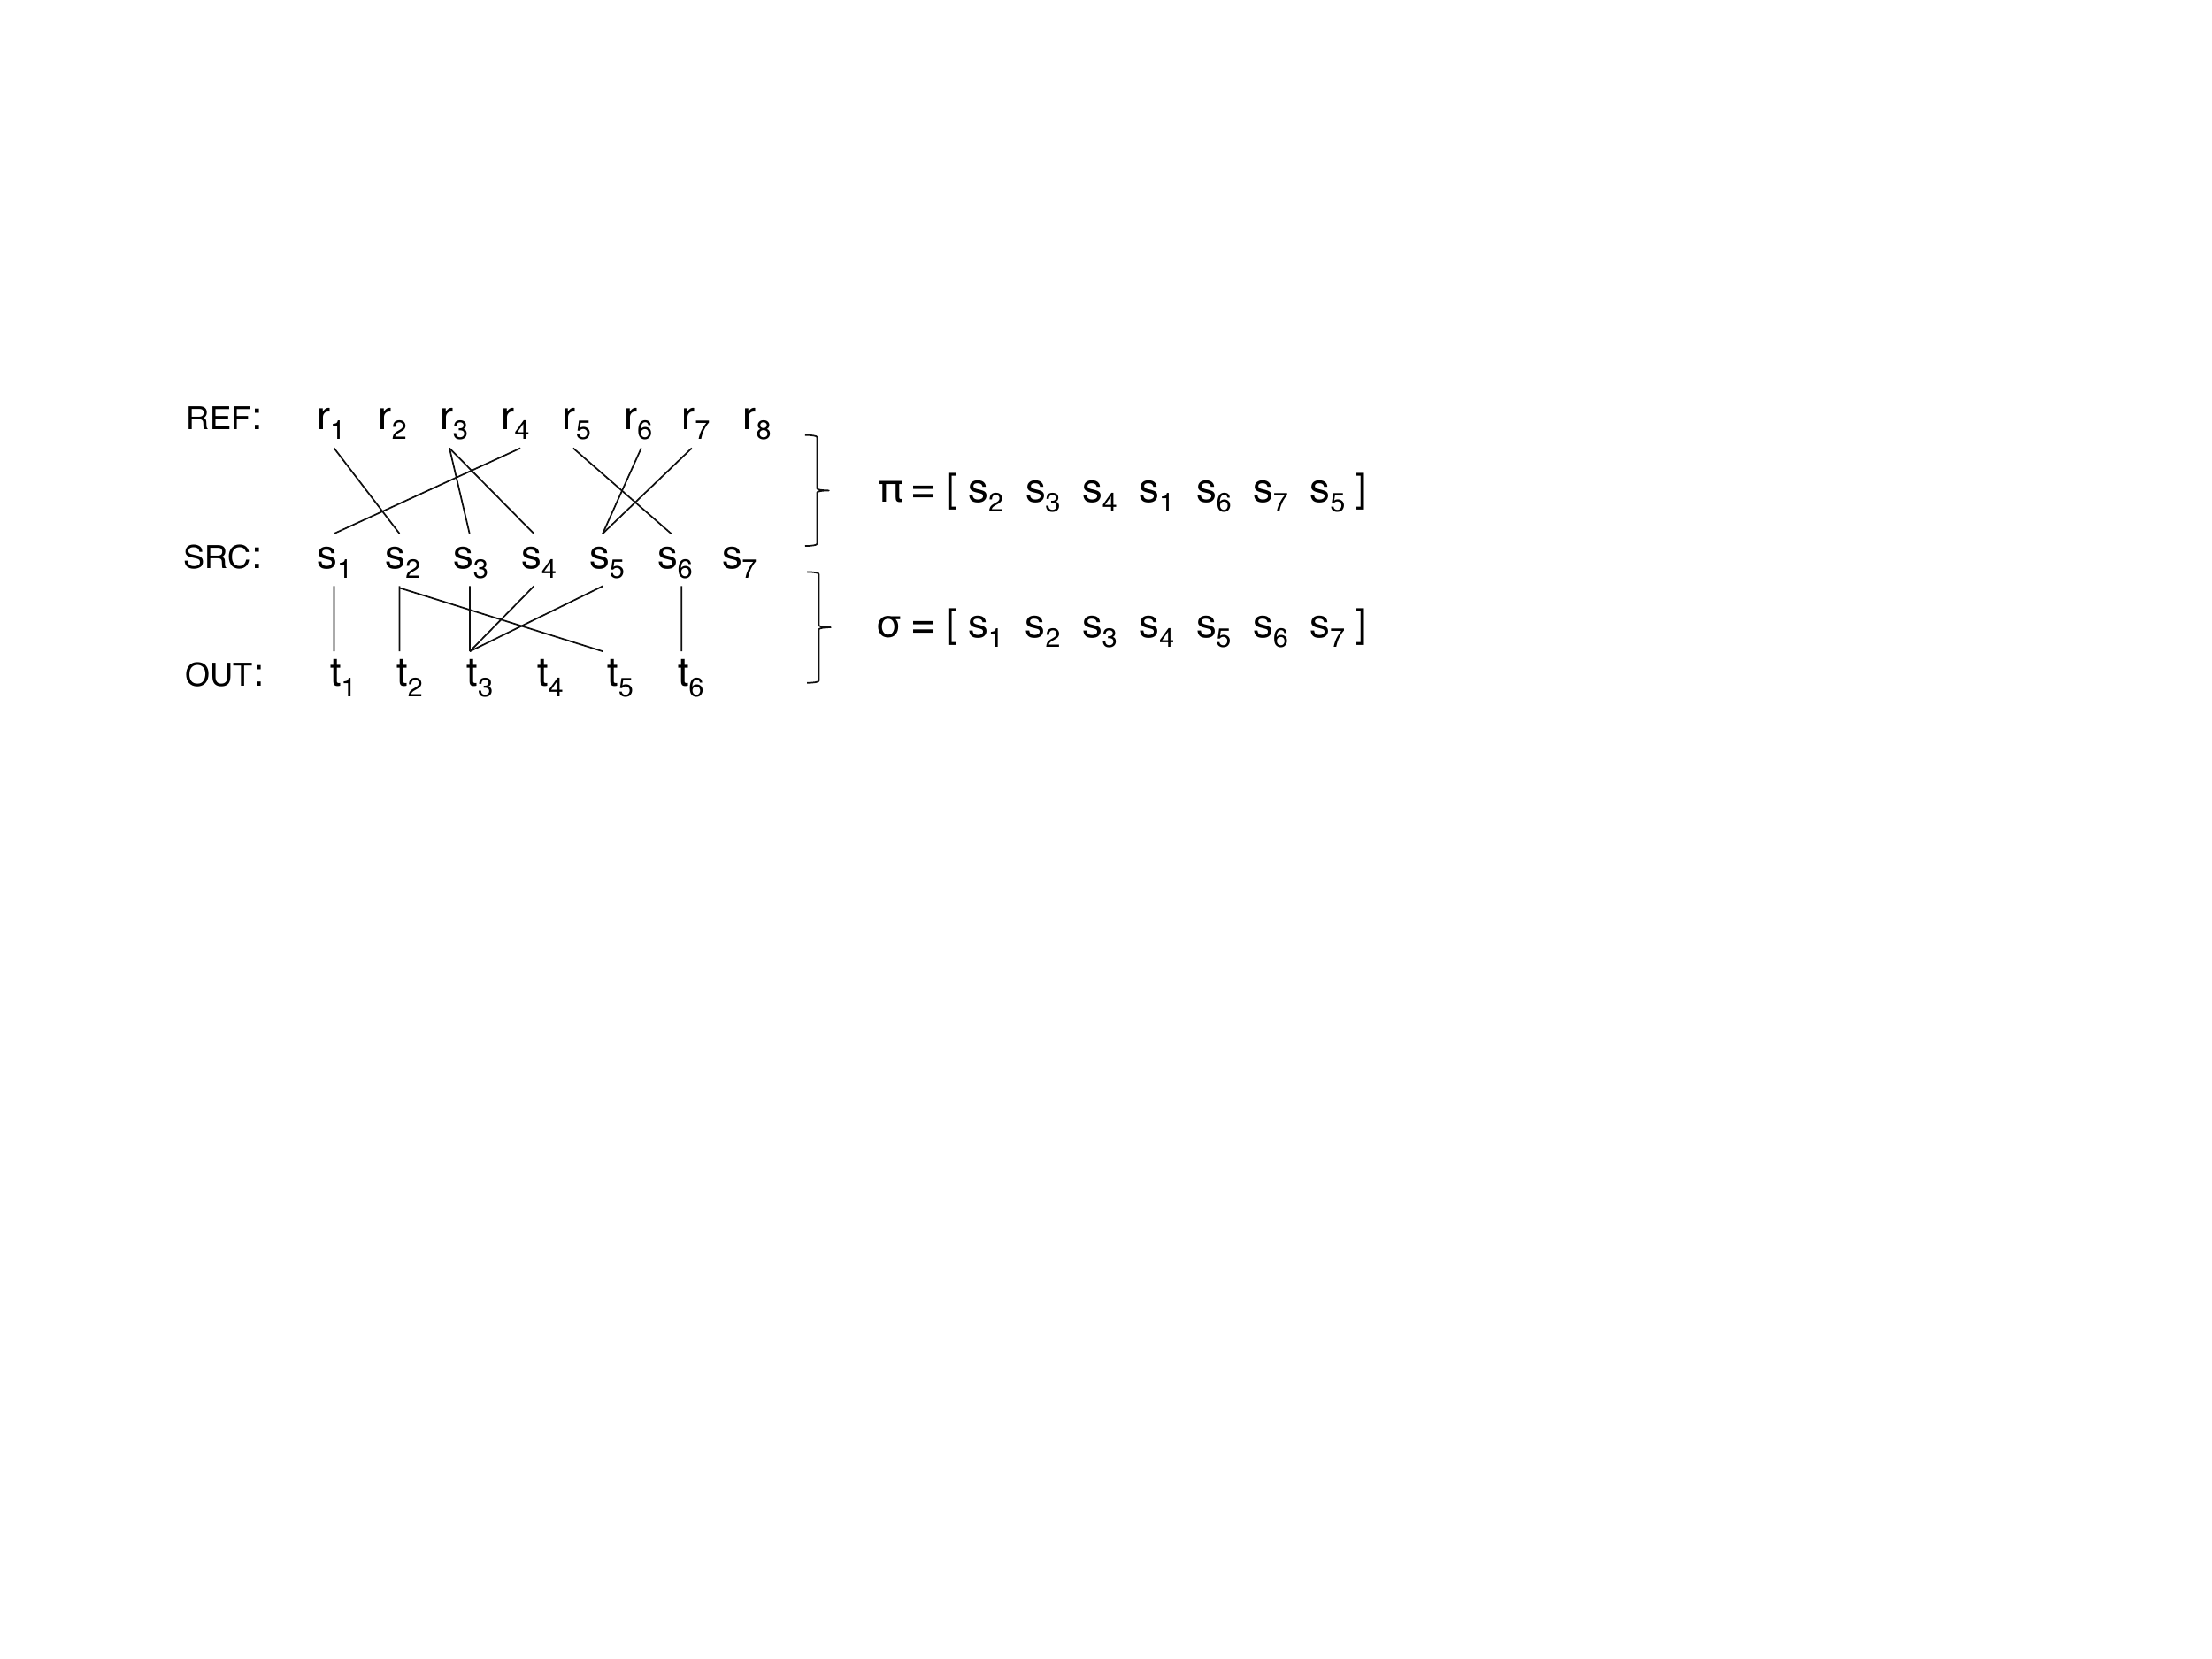}
\caption{\label{fig:KRS} {Example of KRS computation showing how word alignments are converted to permutations.}}
\end{figure}

Figure~\ref{fig:KRS} illustrates an example of KRS computation.
A source sentence of 7 words (in the center) is aligned to 
a reference translation of 8 words and to an MT output of 6.
The two word alignment sets are converted to permutations ($\pi$ and $\sigma$) according to the following rules:
(i)   multiple source words aligned to the same target word are considered to be in monotonic order,
(ii)  non-aligned source words are assumed to immediately follow the previous source word, and 
(iii) if a source word is aligned to non-adjacent words in the target, only the first alignment is retained.
Thus, for example, the link \textsc{s2-t5} is ignored, while \textsc{s7} is inserted right after \textsc{s6} in permutation $\sigma$.
The discordant pairs between $\pi$ and $\sigma$ are \textsc{(s1,s2),(s1,s3),(s1,s4),(s5,s6),(s5,s7)}, hence:
\begin{gather}
\nonumber
K(\pi,\sigma) = \frac{5}{\frac{1}{2}7(7-1)} = 0.2381 \quad  \textrm{,}  \quad BP(\pi,\sigma)=\exp \left(1-\frac{8}{6}\right) =0.7165 \\
\nonumber
KRS = (1-\sqrt{0.2381}) \cdot BP = 0.3669
\end{gather}
\noindent
In the example of Table~\ref{tab:Birch}, 
hypothesis (a) would obtain a much higher KRS than (b): that is 0.8509 versus 0.2546.
